# Supplementary material for: Accelerating Training of Transformer-Based Language Models with Progressive Layer Dropping
Source: arXiv:2010.13369 source file (2020-10-26)
Supplement: Supplementary file 1 [file additional.tex]

\section{Model Architecture Change For Layer-Drop}

One natural way to increase the model capacity is simply increasing the layer number $L$. Unfortunately, Figure~\ref{fig:vanishing-gradients} shows that this would raise gradient vanishing issue at the lower layers. When $L=12$, which is the default layer in the original BERT paper, the gradient vanishing issue exists, but is not severe. However, as we stack more Transformer encoder blocks, the vanishing gradient issue becomes significantly worse. The gradients at the bottom layers are so close to 0 that the learning at those layers becomes close to halt.

% Simply increasing the depth of the model leads to vanishing gradient issue. 

\subsubsection{Revisiting the Transformer networks}

We define Transformer networks as the composition of Transformer blocks, where all Transformer blocks have the same architecture. In particular, a Transformer block consists of two sublayers: a dot-product self-attention layer and a feed-forward layer, with both layers having a skip connection. 
More concretely, for an input $X \in \mathds{R}^{d \times n}$ consisting of d-dimensional embeddings of $n$ tokens, a Transformer block consists of the following two sublayers:

% \begin{equation}
%     Attn(X) = X + \sum_{i=1}^{h}{W_O^i}{W_V^i}X\cdot\sigma[(W_K^iX)^TW_Q^iX] 
% \end{equation}

\begin{equation}
\label{eqn:transformer-self-attention}
\begin{split}
    SL_1(X) &= LayerNorm(X + Attn(X)) \\
            &= LayerNorm(X + {W_O}{W_V}X\cdot softmax[(W_KX)^TW_QX])
\end{split}
\end{equation}

% where $W_O \in \mathds{R}^{}$

% \begin{equation}
%     FF(X) = Attn(X) + W_2\cdot GeLU(W_1\cdot Attn(X) + b_1) + b_2
% \end{equation}

\begin{equation}
\label{eqn:feed-forward}
\begin{split}
    SL_2(X) &= LayerNorm(SL_1(X) + FF(SL_1(X))) \\
            &= LayerNorm(SL_1(X) + W_2\cdot gelu(W_1\cdot SL_1(X)))
\end{split}
\end{equation}

Based on Eqn.~\ref{eqn:transformer-self-attention}--\ref{eqn:feed-forward}, we have for each layer $l$:

\begin{equation}
\label{eqn:analysis-1}
\begin{split}
    X_{l+1} &= LayerNorm(SL_1(X_l) + FF(SL_1(X_l))) \\
            &= LayerNorm(LayerNorm(X_{l} + Attn(X_{l})) + FF(LayerNorm(X_{l} + Attn(X_{l})))) \\
\end{split}
\end{equation}

% Assume $F(X, W) = {W_O}{W_V}X\cdot softmax[(W_KX)^TW_QX]$, then 
% Recursively we will have

% \begin{equation}
% \begin{split}
%     X_{l+2} &= LayerNorm(LayerNorm(X_{l+1} + Attn(X_{l+1})) + FF(LayerNorm(X_{l+1} + Attn(X_{l+1})))) \\
%     & = LayerNorm(LayerNorm(X_{l+1} + F(X_{l+1}))+ W_2(l)\cdot gelu(W_1(l)\cdot LayerNorm(X_{l+1} + F(X_{l+1}))) \\
%     & = ...
% \end{split}
% \end{equation}

% \begin{equation}
% \begin{split}
%     X_{l+2} &= LayerNorm(Attn(X_{l+1}) + W_2(l)\cdot gelu(W_1(l)\cdot Attn(X_{l+1}))) \\
%     & = LayerNorm(LayerNorm(X_{l+1} + F(X_{l+1}))+ W_2(l)\cdot gelu(W_1(l)\cdot LayerNorm(X_{l+1} + F(X_{l+1}))) \\
%     & = ...
% \end{split}
% \end{equation}

% Explain what LayerNorm is used for.

The layer normalization as in \cite{layer-norm} keeps the magnitude of the hidden layers from growing large. As can be seen, the LayerNorm layer alters the signal that passes through the skip connection and impedes information propagation, as reflected by the difficulties on reducing training loss after we increase the model depth (Fig.~\ref{}). Furthermore, SGD and dropout perturb the normalisation, leading to high variance in training error. The effect gets worse with depth, so simply stacking more Transformer blocks tend to perform poorly.

Explain why LayerNorm causes an issue.

% The encoder block passes the input features to a self-attention layer followed by a feed-forward neural network with 1 hidden layer and the ReLU activation function. Before these sub-modules, we follow the original work to include residual connections which establishes short-cuts between the lower-level representation and higher layers. The presence of the residual layers massively increases the magnitude of the neuron values is then alleviated by the layer-normalization layers placed after each residual connection. 

\href{https://arxiv.org/pdf/1911.03179.pdf}{Why Deep Transformers are Difficult to Converge?
From Computation Order to Lipschitz Restricted Parameter Initialization}

"We empirically show
that with proper parameter initialization, deep
Transformers with the original computation order can converge, which is quite in contrast
to all previous works, and obtain significant
improvements with up to 24 layers."

Plot: Gradient norm (y-axis) of each encoder layer (top)
and decoder layer (bottom) in Transformer with respect to layer depth (x-axis).

Show the difference between L12, L24, L48, L72, L101

1. By adding identity mapping, the output x can be thought of as a recursive summation of the outputs from all previous layers. In contrast, without skip connections, then the output is the products of a series of matrix-vector.

2. Gradients at skip connection boundary can be decomposed into two additive terms: a term that propagates information directly without concerning any weight layers, and another term that propagates through the weight layers. The first term ensures that the information is directly propagated back to any shallower unit. 
Another hypothesis is that the second term makes it more unlikely to have vanished gradients (this remains unclear as whether gradients indicate vanish in early layers in BERT, something to verify and potentially can be used to show if skip connections help).

3. Even though additional gating and conv shortcut introduces more parameters and should have a stronger representational abilities than identity shortcuts. Representation ability is not the only factor that decides whether a model behave good or not. There are at least two aspects: optimization issues and representational abilities. 

4. If additional components such as BN are added along the shortcut link, signals are altered before passing to previous layers (which indicates that we should keep the highway clean). 

5. Using asymmetric after-addition activation is equivalent to constructing a pre-activation Residual Unit.

\begin{figure}
    \centering
    \includegraphics[scale=0.4]{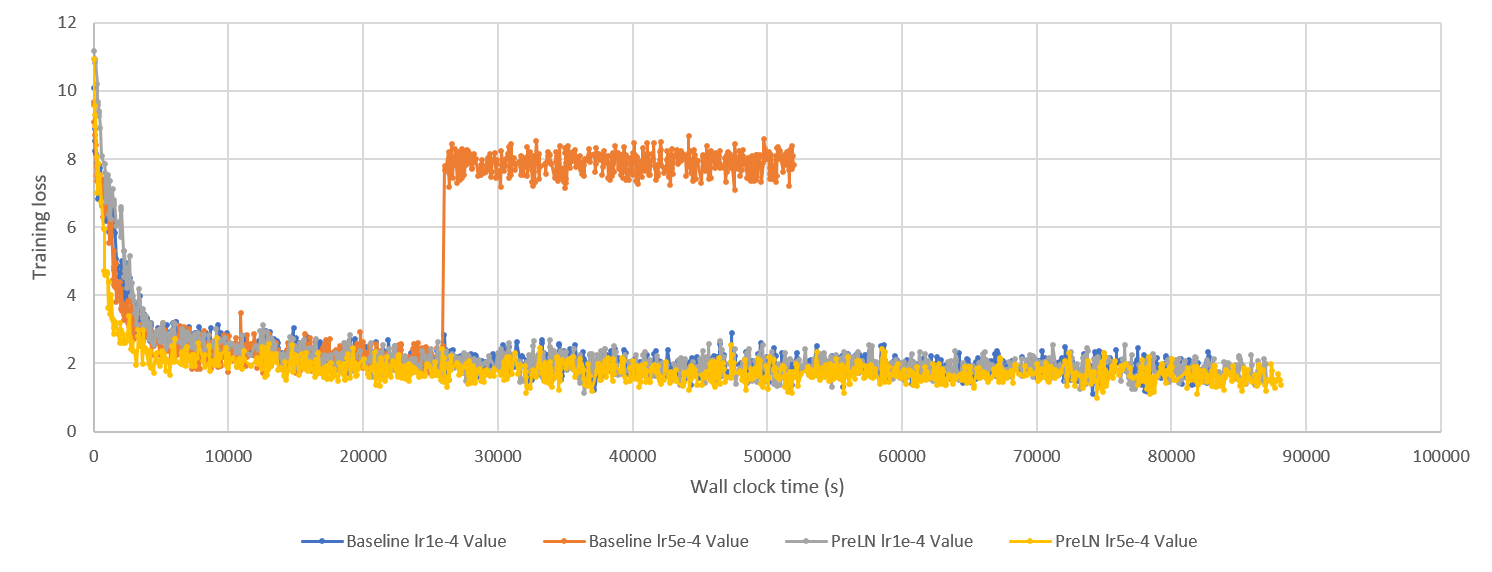}
    \caption{Identity mapping reordering makes training more stable and helps the model to learn with a larger learning rate.}
    \minjia{Add learning rate schedules.}
    \minjia{Add changes of gradient norm before and after identity mapping and with different learning rate. We need fine-grained features to show that "identity mapping has an effect on stabilizing network parameters". Another way is to show the L2 distance and cosine similarity of the input and output embeddings for each layer. Check how Albert shows it with weight sharing.}
    \label{fig:preln-improve-lr}
\end{figure}
